# Supplementary material for: A note on the Eisenbud-Mazur Conjecture
Source: arXiv:1407.5316 ancillary file (2014-07-20)
Supplement: Supplementary file 1 [file appendix_of_computations.pdf]

# Appendix to 'A note on the Eisenbud Mazur conjecture'

July 20, 2014

Here, we provide step by step details for the computations discussed in section 2.6 of the paper.

1.

$$\begin{aligned}
& \operatorname{tr}(g_i^2(x_1+f_1)^2+(x_i+f_i)^2-2g_i((x_1+f_1)(x_i+f_i))) \\
= \;& x_1^2g_i^2+f_1^2g_i^2-2x_1x_ig_i-2f_1f_2g_i+x_i^2+f_i^2 \\
= \;& x_1^2g_i^2+f_1^2g_i^2-2x_1x_ig_i-2f_1^2g_i^2+x_i^2+f_1^2g_i^2 \\
= \;& x_1^2g_i^2-2x_1x_ig_i+x_i^2 \\
= \;& x_1^2g_i^2-x_1x_ig_i-x_1x_ig_i+x_i^2 \\
= \;& x_1g_i(x_1g_i-x_i)-x_i(x_1g_i-x_i) \\
\in \;& \mathfrak{m}P
\end{aligned}$$

2.

$$\begin{aligned}
& \operatorname{tr}(g_i(f_1-x_1)(x_1+f_1)^2+(x_1-f_1)(x_1+f_1)(x_i+f_i)) \\
= \;& -x_1^3g_i+x_1^2f_1g_i-x_1f_1^2g_i+f_1^3g_i+x_1^2x_i-x_1x_if_1+x_1f_1f_i-f_1^2f_i \\
= \;& -x_1^3g_i+x_1^2f_1g_i-x_1f_1^2g_i+f_1^3g_i+x_1^2x_i-x_1x_if_1+x_1f_1^2g_i-f_1^3g_i \\
= \;& -x_1^3g_i+x_1^2x_i+x_1^2f_1g_i-x_1x_if_1 \\
= \;& -x_1^2(x_1g_i-x_i)+x_1f_1(x_1g_i-x_i) \\
\in \;& \mathfrak{m}P
\end{aligned}$$

3.

$$\begin{aligned}
& \operatorname{tr}(g_i g_j (3f_1 - x_1)(x_1+f_1)^2 - 2f_i((x_1+f_1)(x_j+f_j) \\
& +(x_j - f_j)((x_1+f_1)(x_i+f_i)) \\
= \;& -x_1^3 g_i g_j + 3x_1^2 f_1 g_i g_j - x_1 f_1^2 g_i g_j + 3f_1^3 g_i g_j - 2x_1 x_j f_1 g_i \\
& -2f_1^2 f_j g_i - x_1 x_i f_1 g_j - f_1^2 f_i g_j + x_1 x_i x_j + x_j f_1 f_i \\
= \;& -x_1^3 g_i g_j + 3x_1^2 f_1 g_i g_j - x_1 f_1^2 g_i g_j + 3f_1^3 g_i g_j - 2x_1 x_j f_1 g_i \\
& -2f_1^3 g_j g_i - x_1 x_i f_1 g_j - f_1^3 g_i g_j + x_1 x_i x_j + x_j f_1^2 g_i \\
= \;& -x_1^3 g_i g_j + x_1 x_i x_j + 2x_1^2 f_1 g_i g_j - 2x_1 x_j f_1 g_i \\
& +x_1^2 f_1 g_i g_j - x_1 x_i f_1 g_j + x_j f_1^2 g_i - x_1 f_1^2 g_i g_j
\end{aligned}$$

Now, $-x_1^3 g_i g_j + x_1 x_i x_j = -x_1^3 g_j (x_1 g_i - x_i) - x_1 x_i (x_1 g_j - x_j)$. So that,

$$\begin{aligned}
& \operatorname{tr}(g_i g_j (3f_1 - x_1)(x_1+f_1)^2 - 2f_i((x_1+f_1)(x_j+f_j) \\
& +(x_j - f_j)((x_1+f_1)(x_i+f_i)) \\
= \;& -x_1^3 g_j (x_1 g_i - x_i) - x_1 x_i (x_1 g_j - x_j) + 2x_1 f_1 g_i (x_1 g_j - x_j) \\
& +x_1 f_1 g_j (x_1 g_i - x_i) + f_1^2 g_i (x_j - x_1 g_j) \\
\in \;& \mathfrak{m}P
\end{aligned}$$

4.

$$\begin{aligned}
& \operatorname{tr}(g_i g_j (2f_1 - x_1)(x_1+f_1)^2 + x_1(x_i+f_i)(x_j+f_j) \\
& -f_i(x_1+f_1)(x_j+f_j) - f_j(x_1+f_1)(x_i+f_i)) \\
= \;& -x_1^3 g_i g_j + 2x_1^2 f_1 g_i g_j - x_1 f_1^2 g_i g_j + 2f_1^3 g_i g_j + x_1 x_i x_j \\
& -x_1 x_j f_i - x_1 x_i f_j + x_1 f_i f_j - 2f_1 f_i f_j \\
= \;& -x_1^3 g_i g_j + 2x_1^2 f_1 g_i g_j - x_1 f_1^2 g_i g_j + 2f_1^3 g_i g_j + x_1 x_i x_j \\
& -x_1 x_j f_1 g_i - x_1 x_i f_1 g_j + x_1 f_1^2 g_i g_j - 2f_1^3 g_i g_j \\
= \;& -x_1^3 g_i g_j + x_1 x_i x_j + x_1^2 f_1 g_i g_j - x_1 x_i f_1 g_j \\
& +x_1^2 f_1 g_i g_j - x_1 x_j f_1 g_i
\end{aligned}$$

Now, $-x_1^3 g_i g_j + x_1 x_i x_j = -x_1^3 g_j (x_1 g_i - x_i) - x_1 x_i (x_1 g_j - x_j)$. So that,

$$\begin{aligned}
& \operatorname{tr}(g_i g_j (2f_1 - x_1)(x_1+f_1)^2 + x_1(x_i+f_i)(x_j+f_j) \\
& -f_i(x_1+f_1)(x_j+f_j) - f_j(x_1+f_1)(x_i+f_i)) \\
= \;& -x_1^3 g_j (x_1 g_i - x_i) - x_1 x_i (x_1 g_j - x_j) + x_1 f_1 g_j (x_1 g_i - x_i) \\
& +x_1 f_1 g_i (x_1 g_j - x_j) \\
\in \;& \mathfrak{m}P
\end{aligned}$$

5.

$$\begin{aligned}
& \operatorname{tr}(g_i g_j (x_1+f_1)^2 + (x_i+f_i)(x_j+f_j) \\
& -g_i(x_1+f_1)(x_j+f_j) - g_j(x_1+f_1)(x_i+f_i)) \\
= \;& x_1^2 g_i g_j + f_1^2 g_i g_j - x_1 x_j g_i - f_1 f_j g_i - x_1 x_i g_j - f_1 f_i g_j + x_i x_j + f_i f_j \\
= \;& x_1^2 g_i g_j + f_1^2 g_i g_j - x_1 x_j g_i - f_1^2 g_j g_i - x_1 x_i g_j - f_1^2 g_2 g_j + x_i x_j + f_1^2 g_i g_j \\
= \;& x_1^2 g_i g_j - x_1 x_j g_i - x_1 x_i g_j + x_i x_j \\
= \;& x_1 g_i (x_1 g_j - x_j) - x_i (x_1 g_j - x_j) \\
\in \;& \mathfrak{m}P
\end{aligned}$$

6.

$$\begin{aligned}
& \operatorname{tr}(g_i^2 g_j (4f_1 - x_1)(x_1+f_1)^2 + x_i(x_i+f_i)(x_j+f_j) \\
& -f_1 g_i^2 (x_1+f_1)(x_j+f_j) - 3f_1 g_i g_j (x_1+f_1)(x_j+f_j)) \\
= \;& -x_1^3 g_i^2 g_j + 4x_1^2 f_1 g_i^2 g_j - x_1 f_1^2 g_i^2 g_j + 4f_1^3 g_i^2 g_j \\
& -x_1 x_j f_1 g_i^2 - f_1^2 f_j g_i^2 - 3x_1 x_i f_1 g_i g_j - 3f_1^2 f_i g_i g_j \\
& +x_i^2 x_j + x_i f_i f_j \\
= \;& -x_1^3 g_i^2 g_j + 4x_1^2 f_1 g_i^2 g_j - x_1 f_1^2 g_i^2 g_j + 4f_1^3 g_i^2 g_j \\
& -x_1 x_j f_1 g_i^2 - f_1^3 g_j g_i^2 - 3x_1 x_i f_1 g_i g_j - 3f_1^3 g_i^2 g_j \\
& +x_i^2 x_j + x_i f_1^2 g_i g_j \\
= \;& x_i^2 x_j - x_1^3 g_i^2 g_j + x_1^2 f_1 g_i^2 g_j - x_1 x_j f_1 g_i^2 \\
& +3x_1^2 f_1 g_i^2 g_j - 3x_1 x_i f_1 g_i g_j + x_i f_1^2 g_i g_j - x_1 f_1^2 g_i^2 g_j
\end{aligned}$$

Now, $x_i^2 x_j - x_1^3 g_i^2 g_j = -x_1^2 g_j g_i (x_1 g_i - x_i) - x_1 x_i g_j (x_1 g_i - x_i) - x_i^2 (x_1 g_j - x_j)$.
So that,

$$\begin{aligned}
& \operatorname{tr}(g_i^2 g_j (4f_1 - x_1)(x_1+f_1)^2 + x_i(x_i+f_i)(x_j+f_j) \\
& -f_1 g_i^2 (x_1+f_1)(x_j+f_j) - 3f_1 g_i g_j (x_1+f_1)(x_j+f_j)) \\
= \;& (-x_1^2 g_j g_i - x_1 x_i g_j)(x_1 g_i - x_i) - x_i^2 (x_1 g_j - x_j) \\
& +x_1 f_1 g_i^2 (x_1 g_j - x_j) + 3x_1 f_1 g_i g_j (x_1 g_i - x_i) \\
& +f_1^2 g_i g_j (x_i - x_1 g_i) \\
\in \;& \mathfrak{m}P
\end{aligned}$$

7.

$$\begin{aligned}
& \operatorname{tr}(g_i^2 (3f_1 - x_1)(x_1+f_1)^2 + (x_i - 3f_i)(x_1+f_1)(x_i+f_i)) \\
= \;& -x_1^3 g_i^2 + 3x_1^2 f_1 g_i^2 - x_1 f_1^2 g_i^2 + 3f_1^3 g_i^2 - 3x_1 x_i f_1 g_i - 3f_1^2 f_i g_i + x_1 x_i^2 + x_i f_1 f_i \\
= \;& -x_1^3 g_i^2 + 3x_1^2 f_1 g_i^2 - x_1 f_1^2 g_i^2 + 3f_1^3 g_i^2 - 3x_1 x_i f_1 g_i - 3f_1^3 g_i^2 + x_1 x_i^2 + x_i f_1^2 g_i \\
= \;& -x_1^3 g_i^2 + x_1 x_i^2 + 3x_1^2 f_1 g_i^2 - 3x_1 x_i f_1 g_i + x_i f_1^2 g_i - x_1 f_1^2 g_i^2 \\
= \;& -x_1 (x_1 g_i + x_i)(x_1 g_i - x_i) + 3x_1 f_1 g_i (x_1 g_i - x_i) + f_1^2 g_i (x_i - x_1 g_i) \\
\in \;& \mathfrak{m}P
\end{aligned}$$

8.

$$\begin{aligned}
& \operatorname{tr}((g_i(2f_1 - x_1) + x_i)(x_1 + f_1)^2 - 2f_1((x_1 + f_1)(x_i + f_i))) \\
= \quad & -x_1^3 g_i + x_1^2 x_i - 2x_1^2 f_1 g_i + 2x_1^2 f_i - x_1 f_1^2 g_i - x_i f_1^2 + 2x_1 f_1 f_i \\
= \quad & -x_1^3 g_i + x_1^2 x_i - 2x_1^2 f_1 g_i + 2x_1^2 f_1 g_i - x_1 f_1^2 g_i - x_i f_1^2 + 2x_1 f_1^2 g_i \\
= \quad & -x_1^2(g_i x_1 - x_i) + f_1^2(g_i x_1 - x_i) \\
\in \quad & \mathfrak{m}P
\end{aligned}$$

9.

$$\begin{aligned}
& \operatorname{tr}(g_i^3(4f_1 - x_1)(x_1 + f_1)^2 + x_i(x_i + f_i)^2 - 4f_1 g_i^2(x_1 + f_1)(x_i + f_i)) \\
= \quad & -x_1^3 g_i^3 + 4x_1^2 f_1 g_i^3 - x_1 f_1^2 g_i^3 + 4f_1^3 g_i^3 - 4x_1 x_i f_1 g_i^2 - 4f_1^2 f_i g_i^2 + x_i^3 + x_i f_i^2 \\
= \quad & -x_1^3 g_i^3 + 4x_1^2 f_1 g_i^3 - x_1 f_1^2 g_i^3 + 4f_1^3 g_i^3 - 4x_1 x_i f_1 g_i^2 - 4f_1^3 g_i^3 + x_i^3 + x_i f_1^2 g_i^2 \\
= \quad & x_i^3 - x_1^3 g_i^3 - x_1 f_1^2 g_i^3 + x_i f_1^2 g_i^2 + 4x_1^2 f_1 g_i^3 - 4x_1 x_i f_1 g_i^2 \\
= \quad & (x_i - x_1 g_i)(x_i^2 + x_1 x_i g_i + x_1^2 g_i^2) - f_1^2 g_i^2(x_1 g_i - x_i) + 4x_1 f_1 g_i^2(x_1 g_i - x_i) \\
\in \quad & \mathfrak{m}P
\end{aligned}$$

10.

$$\begin{aligned}
& \operatorname{tr}(g_i^2(2f - x_1)(x_1 + f_1)^2 + x_1(x_i + f_i)^2 - 2f_i((x_1 + f_1)(x_i + f_i))) \\
= \quad & -x_1^3 g_i^2 - x_1 f_1^2 g_i^2 + 2x_1^2 f_i g_i + 2f_1^2 f_i g_i + x_1 x_i^2 - 2x_1 x_i f_i + x_1 f_i^2 - 2f_1 f_i^2 \\
= \quad & -x_1^3 g_i^2 - x_1 f_1^2 g_i^2 + 2x_1^2 f_1 g_i^2 + 2f_1^3 g_i^2 + x_1 x_i^2 - 2x_1 x_i f_1 g_i + x_1 f_1^2 g_i^2 - 2f_1^3 g_i^2 \\
= \quad & -x_1^3 g_i^2 + x_1 x_i^2 - 2x_1 x_i f_1 g_i + 2x_1^2 f_1 g_i^2 \\
= \quad & -x_1(x_1 g_i + x_i)(x_1 g_i - x_i) - 2x_1 f_1 g_i(x_i - x_1 g_i) \\
\in \quad & \mathfrak{m}P
\end{aligned}$$

11.

$$\begin{aligned}
& \operatorname{tr}(g_i^2 g_j(4f_1 - x_1)(x_1 + f_1)^2 + x_j(x_i + f_i)^2 \\
& -2f_1 g_i^2(x_1 + f_1)(x_j + f_j) - 2f_1 g_i g_j(x_1 + f_1)(x_i + f_i)) \\
= \quad & -x_1^3 g_i^2 g_j + 4x_1^2 f_1 g_i^2 g_j - x_1 f_1^2 g_i^2 g_j \\
& +4f_1^3 g_i^2 g_j - 2x_1 x_j f_1 g_i^2 - 2f_1^2 f_j g_i^2 - 2x_1 x_i f_1 g_i g_j \\
& -2f_1^2 f_i g_i g_j + x_i^2 x_j + x_j f_i^2 \\
= \quad & -x_1^3 g_i^2 g_j + 4x_1^2 f_1 g_i^2 g_j - x_1 f_1^2 g_i^2 g_j \\
& +4f_1^3 g_i^2 g_j - 2x_1 x_j f_1 g_i^2 - 2f_1^3 g_j g_i^2 - 2x_1 x_i f_1 g_i g_j \\
& -2f_1^3 g_i^2 g_j + x_i^2 x_j + x_j f_1^2 g_i^2 \\
= \quad & -x_1^3 g_i^2 g_j + x_i^2 x_j - x_1 f_1^2 g_i^2 g_j + x_j f_1^2 g_i^2 \\
& +2x_1^2 f_1 g_i^2 g_j - 2x_1 x_j f_1 g_i^2 + 2x_1^2 f_1 g_i^2 g_j - 2x_1 x_i f_1 g_i g_j
\end{aligned}$$

Now, $-x_1^3g_i^2g_j+x_i^2x_j = -x_1^2g_ig_j(x_1g_i-x_i)-x_1x_ig_j(x_1g_i-x_i)-x_i^2(x_1g_j-x_j)$. So that,

$$\begin{aligned}
& \operatorname{tr}(g_i^2g_j(4f_1-x_1)(x_1+f_1)^2+x_j(x_i+f_i)^2 \\
& -2f_1g_i^2(x_1+f_1)(x_j+f_j)-2f_1g_ig_j(x_1+f_1)(x_i+f_i)) \\
= & -x_1^2g_ig_j(x_1g_i-x_i)-x_1x_ig_j(x_1g_i-x_i)-x_i^2(x_1g_j-x_j) \\
& -f_1^2g_i^2(x_1g_j-x_j)+2x_1f_1g_i^2(x_1g_j-x_j) \\
& +2x_1f_1g_ig_j(x_1g_i-x_i) \\
\in & \ \mathfrak{m}P
\end{aligned}$$

12.

$$\begin{aligned}
& \operatorname{tr}(g_ig_jg_k(2f_1-x_1)(x_1+f_1)^2+x_k(x_i+f_i)(x_j+f_j) \\
& -f_1g_j(x_k+f_k)(x_i+f_i)-f_1g_j(x_k+f_k)(x_j+f_j)) \\
= & -x_1^3g_ig_jg_k+2x_1^2f_1g_1g_jg_k-x_1f_1^2g_ig_jg_k+2f_1^3g_ig_jg_k \\
& +x_ix_jx_k-f_ix_jx_k-f_jx_ix_k+f_if_jx_k-2f_if_jf_k \\
= & -x_1^3g_ig_jg_k+2x_1^2f_1g_1g_jg_k-x_1f_1^2g_ig_jg_k+2f_1^3g_ig_jg_k \\
& +x_ix_jx_k-f_1g_ix_jx_k-f_1g_jx_ix_k+f_1^2g_ig_jx_k-2f_1^3g_ig_jg_k \\
= & -x_1^3g_ig_jg_k+x_ix_jx_k-x_1f_1^2g_ig_jg_k+f_1^2g_ig_jx_k \\
& +x_1^2f_1g_1g_jg_k-f_1g_ix_jx_k+x_1^2f_1g_1g_jg_k-f_1g_jx_ix_k
\end{aligned}$$

Now, $-x_1^3g_ig_jg_k+x_ix_jx_k = -x_1^2g_ig_j(x_1g_k-x_k)-x_1x_kg_i(x_1g_j-x_j)-x_jx_k(x_1g_i-x_i)$. Also, $x_1^2f_1g_1g_jg_k-f_1g_ix_jx_k = f_1g_ig_jx_1(x_1g_k-x_k)+f_1g_ix_k(x_1g_j-x_j)$. Finally, $x_1^2f_1g_1g_jg_k-f_1g_jx_ix_k = f_1g_ig_jx_1(x_1g_k-x_k)+f_1g_jx_k(x_1g_i-x_i)$. So that,

$$\begin{aligned}
& \operatorname{tr}(g_ig_jg_k(2f_1-x_1)(x_1+f_1)^2+x_k(x_i+f_i)(x_j+f_j) \\
& -f_1g_j(x_k+f_k)(x_i+f_i)-f_1g_j(x_k+f_k)(x_j+f_j)) \\
= & -x_1^2g_ig_j(x_1g_k-x_k)-x_1x_kg_i(x_1g_j-x_j)-x_jx_k(x_1g_i-x_i) \\
& -f_1^2g_ig_j(x_1g_k-x_k)+f_1g_ig_jx_1(x_1g_k-x_k)+f_1g_ix_k(x_1g_j-x_j) \\
& +f_1g_ig_jx_1(x_1g_k-x_k)+f_1g_jx_k(x_1g_i-x_i) \\
\in & \ \mathfrak{m}P
\end{aligned}$$

Lastly, we need to show the generators of $(Q_1^2\cap Q_2^2)\cap S$ arising by applying the trace map to $Q_1^2Q_2^2$ also lie in $\mathfrak{m}P$. We have, $Q_1^2Q_2^2 = \{(x_i-f_i)(x_j-f_j)(x_{i'}+f_{i'})(x_{j'}+f_{j'}) : i,i^{'},j,j^{'}\in\{1,...,m\}\}$.

We have,

$$
\begin{aligned}
& \operatorname{tr}((x_i - f_i)(x_j - f_j)(x_{i'} + f_{i'})(x_{j'} + f_{j'})) \\
= \; & x_i x_{i'} x_j x_{j'} + f_i f_{i'} x_j x_{j'} + x_i x_{i'} f_j f_{j'} - f_i x_{i'} f_j x_{j'} \\
& - f_i x_{i'} x_j f_{j'} - x_i f_{i'} f_j x_{j'} - x_i f_{i'} x_j f_{j'} + f_i f_{i'} f_j f_{j'} \\
= \; & x_i x_{i'} x_j x_{j'} - f_i x_{i'} f_j x_{j'} + f_i f_{i'} x_j x_{j'} - x_i f_{i'} f_j x_{j'} \\
& + x_i x_{i'} f_j f_{j'} - f_i x_{i'} x_j f_{j'} - x_i f_{i'} x_j f_{j'} + f_i f_{i'} f_j f_{j'} \\
= \; & x_{i'} x_{j'} (x_i x_j - f_i f_j) + f_i f_{i'} x_j x_{j'} - x_i f_{i'} f_j x_{j'} \\
& + x_i x_{i'} f_j f_{j'} - f_i x_{i'} x_j f_{j'} - f_{i'} f_{j'} (x_i x_j - f_i f_j) \\
= \; & x_{i'} x_{j'} (x_i x_j - f_i f_j) + f_i f_{i'} x_j x_{j'} - x_i x_{i'} x_j x_{j'} + x_i x_{i'} x_j x_{j'} - x_i f_{i'} f_j x_{j'} \\
& + x_i x_{i'} f_j f_{j'} - x_i x_{i'} x_j x_{j'} + x_i x_{i'} x_j x_{j'} - f_i x_{i'} x_j f_{j'} - f_{i'} f_{j'} (x_i x_j - f_i f_j \\
= \; & x_{i'} x_{j'} (x_i x_j - f_i f_j) + x_j x_{j'} (f_i f_{i'} - x_i x_{i'}) + x_i x_{j'} (x_{i'} x_j - f_{i'} f_j) \\
& + x_i x_{i'} (f_j f_{j'} - x_j x_{j'}) + x_{i'} x_j (x_i x_{j'} - f_i f_{j'}) - f_{i'} f_{j'} (x_i x_j - f_i f_j) \\
\in \; & \mathfrak{m} P
\end{aligned}
$$
